# Supplementary material for: Phase-Resolved Ultra-High-Energy Emission Defines an Energetic Boundary for Compact-Object Engines and Dense-Matter Structure
Source: arXiv:2609.08824 source file (2026-10-02)
Supplement: Supplementary file 1 [file suplementar.tex]

% ======================================================================
%  SUPPLEMENTAL MATERIAL
%  "Phase-Resolved Ultra-High-Energy Emission as an Orbital Sieve
%   for Dense-Matter Equations of State"
%
%  Compile with the SAME revtex4-2 preamble as the Letter.
%  Two ways to attach it:
%   (A) Separate file: start a fresh document with the preamble below.
%   (B) Same PDF: paste everything BETWEEN the two %%% markers right
%       after \end{acknowledgments}, replacing the standalone wrapper.
%
%  All numbers below are taken verbatim from the 21A robustness run
%  over the full library (124 EoS x 3 scenarios x 3 seeds =
%  6.696e11 explicit Monte Carlo events).
% ======================================================================

\documentclass[aps,prl,twocolumn,superscriptaddress,nofootinbib]{revtex4-2}
\usepackage{amsmath,amssymb}
\usepackage{graphicx}
\usepackage{booktabs}
\usepackage{siunitx}
\begin{document}

%%% ----- BEGIN SUPPLEMENTAL (paste from here if using option B) -----

\newpage
\appendix
\onecolumngrid
\begin{center}
{\bf\large Supplemental Material}\\[2pt]
{\bf\large Phase-Resolved Ultra-High-Energy Emission Defines an Energetic Boundary\\
for Compact-Object Engines and Dense-Matter Structure}\\[4pt]
Marlon M.\ S.\ Mendes and C\'esar H.\ Lenzi
\end{center}
\twocolumngrid

% Requires \usepackage{xcolor} in the main manuscript preamble.
This Supplemental Material provides the derivations, numerical audits,
and consistency tests supporting the construction and results presented
in the main text. Section~\ref{sm:architecture} documents the causal
separation and certified EoS cohort; Sec.~\ref{sm:boundaries} derives
the UHE energetic boundary and circumstellar interaction requirement;
Sec.~\ref{sm:uncertainty} gives the statistical and instrumental
uncertainty treatment; Sec.~\ref{sm:robustness} establishes the
spin-down provenance and mass dependence; Sec.~\ref{sm:closure}
provides the GeV engine-closure test; Sec.~\ref{sm:structural_overlap}
documents the energetic--tidal intersection; and
Sec.~\ref{sm:microphysics} specifies the structural and microphysical
quantities displayed in Fig.~\ref{fig:uhe_boundary_structure}.

% ============================================================
\section{Causal architecture and certified EoS cohort}
\label{sm:architecture}

The analysis is organized so that orbital propagation, source
energetics, and dense-matter diagnostics remain causally separated.
The orbital calculation requires
\begin{equation}
\frac{E_{\max}}{E_{\rm req}}>1,
\qquad
\tau_{\gamma\gamma}(100~{\rm TeV})<1,
\end{equation}
and defines
\begin{equation}
f_{\rm joint}
=
P\!\left[
E_{\max}/E_{\rm req}>1
\cap
\tau_{\gamma\gamma}(100~{\rm TeV})<1
\right].
\end{equation}

The orbital kernel is source-side only: the same phase-resolved Monte
Carlo realizations determine the orbital separation and shock location,
shock magnetic field, wind density and momentum balance, and the
radiation-field geometry entering \(E_{\max}/E_{\rm req}\) and
\(\tau_{\gamma\gamma}\). These quantities define an orbital viability
diagnostic, not an EoS likelihood.

No TOV, Love, radius, tidal-deformability, or sound-speed observable
modifies either orbital condition. Dense matter enters only through
the stellar moment of inertia,
\begin{equation}
{\rm EoS}
\longrightarrow
I(M)
\longrightarrow
\dot E_{\rm sd}
=
4\pi^2 I(M)\frac{\dot P_{\rm rot}}{P^3}.
\label{eq:sm_chain}
\end{equation}
Radius and tidal information are applied only as independent
downstream diagnostics. In particular, no structural score is
multiplied into the UHE energetic boundary.

The upstream inventory contains 175 input EoS realizations. After
source reload, physical validation, full support on the target-mass
axis, branch-resolution checks, and removal of mass-gap cases, the
certified cohort contains 116 EoS. All 116 have native support over the
mass interval used here, a single certified stable branch throughout
that interval, and no target-mass gap. The final branch-resolved data
contain 861 direct stellar nodes. Neither a target EoS count nor a
branch prior is used in constructing the cohort.
The cohort is used as a heterogeneous working library rather than as
independent draws from an EoS population; no permutation significance
test or family-level multiplicity weighting is used.

The stellar sequences are computed with the corrected,
perturbation-decoupled TOV--Love--Hartle implementation used throughout
the analysis. The tidal perturbation is integrated independently of
the rotational sector, with the corrected tidal-sign convention, so
that the moment of inertia and tidal observables are obtained from
their respective perturbative systems rather than through a coupled
numerical prescription.

Direct target-mass reconstruction gives a maximum
\[
|M_{\rm direct}-M_{\rm target}|
\simeq2.1\times10^{-7}\,M_\odot .
\]
The maximum interpolation discrepancies in the certified handoff are
approximately \(0.20\%\) in \(I\), \(0.09\%\) in \(R\), and \(0.72\%\)
in the diagnostic tidal quantity. These values quantify numerical
consistency of the reconstruction and are not observational
uncertainties.

These certified sequences provide the \(I(M)\) values entering the
energetic boundary below. The corresponding \(R(M)\) and
\(\Lambda(M)\) sequences are retained only for the independent
downstream structural comparison in
Sec.~\ref{sm:structural_overlap}.
The orbital Monte Carlo uses the same source-side parameter ranges
adopted in the phase-resolved calculation underlying Fig.~2, including
the orbital separation, shock position and magnetic field, wind
momentum balance, and stellar radiation-field geometry. The
acceleration threshold is evaluated from the resulting maximum
particle energy, while the \(100\) TeV transparency condition is
obtained from the line-of-sight \(\gamma\gamma\) optical depth.
These source parameters are sampled independently of the EoS cohort
and are not adjusted according to \(I\), \(R\), \(\Lambda\), or
\(c_s^2\).

% ============================================================
\section{UHE energetic boundary}
\label{sm:boundaries}

For the hadronic component,
\begin{equation}
L_\gamma^{\rm UHE}
=
q_\gamma\,\xi_p\,f_{pp}\,\dot E_{\rm sd},
\label{eq:sm_lgamma}
\end{equation}
where the baseline neutral-pion energy fraction is
\(q_\gamma=1/3\). The required proton efficiency is
\begin{equation}
\xi_{p,\rm crit}
=
\frac{L_\gamma^{\rm UHE}P^3}
{4\pi^2 q_\gamma I(M)\dot P_{\rm rot}f_{pp}},
\label{eq:sm_xicrit}
\end{equation}
and the energetic boundary is equivalently
\begin{equation}
\dot P_{\rm crit}
=
\frac{L_\gamma^{\rm UHE}P^3}
{4\pi^2 q_\gamma I(M)f_{pp}},
\qquad
I_{\rm crit}
=
\frac{L_\gamma^{\rm UHE}P^3}
{4\pi^2 q_\gamma \dot P_{\rm rot}f_{pp}}.
\label{eq:sm_crit}
\end{equation}

Collecting the EoS-independent source and environmental factors,
\begin{equation}
K_{\rm src}
\equiv
\frac{L_\gamma^{\rm UHE}P^3}
{4\pi^2 q_\gamma f_{pp}},
\label{eq:sm_ksrc}
\end{equation}
the boundary at fixed source conditions becomes
\begin{equation}
\dot P_{{\rm crit},i}(M)
=
\frac{K_{\rm src}}{I_i(M)}.
\label{eq:sm_inverseI}
\end{equation}
All EoS dependence of the energetic ordering is therefore contained
in \(I_i(M)\).

The fiducial value \(q_\gamma=1/3\) is a physical conversion assumption,
not a fitted coefficient; \(q_\gamma=1/4\) is retained only as an
explicit stress test.

The effective proton--proton interaction fraction is
\begin{equation}
f_{pp}
=
\frac{t_{\rm esc}}{t_{pp}+t_{\rm esc}},
\qquad
t_{pp}^{-1}
=
n\kappa_{pp}\sigma_{pp}c .
\label{eq:sm_fpp}
\end{equation}
At \(\xi_{p,\rm crit}=1\),
\begin{align}
f_{pp,\min}
&=
\frac{L_\gamma^{\rm UHE}P^3}
{4\pi^2 q_\gamma I(M)\dot P_{\rm rot}},
\\
n_{\min}
&=
\frac{f_{pp,\min}}
{(1-f_{pp,\min})
 \kappa_{pp}\sigma_{pp}c\,t_{\rm esc}}.
\label{eq:sm_nmin}
\end{align}
Therefore, for a fixed energetic requirement,
\begin{equation}
n_{\min}t_{\rm esc}={\rm const.},
\end{equation}
so the physical requirement is an interaction-depth condition rather
than a density-only condition.
The reference environmental values
\(\kappa_{pp}=0.5\), \(\sigma_{pp}=40~{\rm mb}\), and
\(t_{\rm esc}=10^3~{\rm s}\) are fixed independently of the EoS cohort
and are not optimized to place the boundary inside the physical
\(I(M)\) distribution. The density ceiling is therefore a source-side
stress boundary rather than a measured density; its dependence is
explicit in Eqs.~(\ref{eq:sm_fpp})--(\ref{eq:sm_nmin}) and in
Sec.~\ref{sm:uncertainty}. These values give \(f_{pp}=0.05657\) at
\(n=10^{11}~{\rm cm^{-3}}\) and \(f_{pp}=0.53254\) at
\(n=1.9\times10^{12}~{\rm cm^{-3}}\).
For either spectral construction, the observed energy flux is converted
to isotropic-equivalent luminosity through
\begin{equation}
L_\gamma(d)=4\pi d^2 F_\gamma .
\label{eq:sm_flux_lum}
\end{equation}

For the measured \(25\)--\(100\) TeV tail,
\begin{equation}
F_{25-100}
=
1.05\times10^{-13}
~{\rm erg\,cm^{-2}\,s^{-1}},
\end{equation}
which corresponds at 2.0 kpc to
\begin{equation}
L_{\gamma,25-100}
=
5.03\times10^{31}
~{\rm erg\,s^{-1}}.
\end{equation}
Using the current certified median
\(I_{45}(1.4)=1.7161\) and
\(\dot P_{\rm ref}=3\times10^{-15}~{\rm s\,s^{-1}}\),
Eq.~(\ref{eq:sm_nmin}) gives
\begin{equation}
n_{\min}(2.0~{\rm kpc})
=
2.45\times10^{10}~{\rm cm^{-3}},
\end{equation}
and
\begin{equation}
n_{\min}(2.65~{\rm kpc})
=
4.35\times10^{10}~{\rm cm^{-3}}.
\end{equation}
These values supersede thresholds obtained with the earlier
moment-of-inertia library.

The pure-hadronic \(>1\) TeV construction is not adopted as the preferred
emission model. It is a deliberately demanding limiting stress test
used to determine when the source-energy requirement enters the
physical \(I(M)\) range.
For this case, the direct spectral integration gives
\begin{equation}
F_{E>1{\rm TeV}}
=
3.493\times10^{-12}
~{\rm erg\,cm^{-2}\,s^{-1}},
\end{equation}
or
\begin{equation}
L_{\gamma,>1{\rm TeV}}(2~{\rm kpc})
=
1.672\times10^{33}
~{\rm erg\,s^{-1}}.
\end{equation}
At the disk-density ceiling,
\begin{equation}
L_{p,\rm req}
=
\frac{L_{\gamma,>1{\rm TeV}}}
{q_\gamma f_{pp}}
=
9.42\times10^{33}
~{\rm erg\,s^{-1}},
\end{equation}
and the corresponding canonical-mass crossing is
\begin{equation}
I_{45,\rm crit}=1.5504.
\label{eq:sm_icrit}
\end{equation}
This value follows the direct spectral chain above; rounded luminosity
chains are not mixed into the quoted crossing.

These quantities define the source-dependent boundary whose uncertainty
and mass dependence are quantified in
Secs.~\ref{sm:uncertainty} and \ref{sm:robustness}.

% ============================================================
\section{Statistical and instrumental uncertainty contract}
\label{sm:uncertainty}
The source-statistical propagation uses \(10^7\) draws of the LHAASO
spectral normalization and index, split across three independent
random seeds. The baseline spectral inputs are
\begin{equation}
N_0=(2.18\pm0.20)\times10^{-15}
~{\rm TeV^{-1}\,cm^{-2}\,s^{-1}}
\end{equation}
at 10 TeV and
\begin{equation}
\Gamma=3.00\pm0.05.
\end{equation}
Because a published \(N_0\)--\(\Gamma\) covariance is not available,
the statistical baseline uses zero covariance; this is a bookkeeping
assumption, not a claim of physical independence.
For the pure-hadronic \(>1\) TeV boundary, the statistical
\(N_0,\Gamma\) propagation gives 16th, 50th, and 84th percentile
multiplicative factors \(0.891,\ 0.999,\) and \(1.115\) in
\(\dot P_{\rm crit}\). For the cohort-median 2.0-kpc,
\(1.4\,M_\odot\) boundary, these correspond to
\((2.42,\ 2.71,\ 3.02)\times10^{-15}~{\rm s\,s^{-1}}\),
respectively.


Instrumental calibration uncertainties are not sampled as probability
priors. They are represented by seven coherent bounded states covering
the quoted WCDA flux-scale uncertainty, the additional WCDA spatial
model uncertainty, the KM2A flux-scale uncertainty, and the KM2A
spectral-index shift. The KM2A \(\Delta\Gamma\) state is applied only
to the KM2A energy domain. Thus the calibration result is an envelope,
not a posterior probability distribution.

The \(10^7\)-draw calculation is numerically converged relative to the
earlier \(3\times10^6\)-draw run: the maximum change in any conditional
energy fraction is \(3.4\times10^{-4}\), the largest seed-to-seed
standard deviation is \(5.9\times10^{-4}\), and the mass-quadrature
change between 1001 and 2001 mass points is
\(2.3\times10^{-7}\). These numerical uncertainties are much smaller
than the physical uncertainty associated with the unknown intrinsic
\(\dot P_{\rm rot}\).

At \(M=1.4\,M_\odot\), the cohort-median critical boundaries and their
coherent instrumental envelopes are
\begin{equation}
\begin{array}{lll}
{\rm mixed},~2.0~{\rm kpc}:&
1.229^{+0.371}_{-0.295}\times10^{-15},\\
{\rm mixed},~2.65~{\rm kpc}:&
2.158^{+0.652}_{-0.518}\times10^{-15},\\
{\rm pure},~2.0~{\rm kpc}:&
2.710^{+0.819}_{-0.651}\times10^{-15},\\
{\rm pure},~2.65~{\rm kpc}:&
4.758^{+1.437}_{-1.143}\times10^{-15},
\end{array}
\end{equation}
in units of \({\rm s\,s^{-1}}\).
The corresponding mass dependence is shown in
Fig.~\ref{fig:uhe_boundary_structure}(b).

For interpretation, we use the absolute logarithmic sensitivity
\begin{equation}
{\cal S}_x
=
\left|
\frac{\partial\ln\dot P_{\rm crit}}
{\partial\ln x}
\right|.
\end{equation}
The pure-hadronic boundary gives exactly
\begin{equation}
{\cal S}_P=3,
\qquad
{\cal S}_d=2,
\qquad
{\cal S}_{I}=1,
\qquad
{\cal S}_{q_\gamma}=1.
\end{equation}
At the disk-density ceiling,
\begin{equation}
{\cal S}_{n}
=
{\cal S}_{t_{\rm esc}}
=
{\cal S}_{\kappa_{pp}}
=
{\cal S}_{\sigma_{pp}}
=
1-f_{pp}
=
0.4675.
\end{equation}
For the mixed construction the direct decomposition gives
\begin{equation}
{\cal S}_{q_\gamma}=0.6242,
\qquad
{\cal S}_{D_p}=0.6242,
\end{equation}
\begin{equation}
{\cal S}_{F_{25-100}}=0.6242,
\qquad
{\cal S}_{F_{1-25}}=
{\cal S}_{f_{\rm IC}}=0.3758,
\end{equation}
and
\begin{equation}
{\cal S}_{n}
=
{\cal S}_{t_{\rm esc}}
=
{\cal S}_{\kappa_{pp}}
=
{\cal S}_{\sigma_{pp}}
=
0.5889.
\end{equation}
These derivatives are interpretation diagnostics only; they are never
used as ranking weights.
The shaded bands in Fig.~\ref{fig:uhe_boundary_structure}(b) show the
EoS spread at the central spectral parameters; the statistical
\(N_0,\Gamma\) propagation and coherent instrumental envelopes above
are separate. Panel (c) shows the logarithmic sensitivities.
% ============================================================
\section{Spin-down provenance and mass dependence}
\label{sm:robustness}

FAST measures
\begin{equation}
P=269.15508\pm0.00016~{\rm ms}
\end{equation}
\cite{Weng2022}, and this value is used throughout the energetic
calculation. Its fractional uncertainty is negligible here.

The same data yield an apparent folding derivative
\begin{equation}
\dot P_{\rm app}
=
(4.2\pm1.2)\times10^{-10}
~{\rm s\,s^{-1}},
\end{equation}
but this is not a phase-connected intrinsic timing measurement.
Binary acceleration contributes
\begin{equation}
\dot P_{\rm orb}=P\,a_\parallel/c,
\end{equation}
and representative orbital accelerations naturally reach the scale
of the reported apparent derivative. Detailed orbital estimates also
show that Doppler contamination can be substantial
\cite{Suvorov2022}. We therefore do not identify
\(\dot P_{\rm app}\) with the rotation-powered spin-down rate.

The value
\begin{equation}
\dot P_{\rm ref}
=
3\times10^{-15}
~{\rm s\,s^{-1}}
\end{equation}
is retained only as a benchmark used in the LHAASO source discussion
\cite{LHAASOLSI}; it is not treated as a measured intrinsic derivative.

The mass dependence follows directly from \(I(M)\). For the cohort
median, the central critical boundaries are
\begin{equation}
\begin{array}{c|ccc}
&1.4\,M_\odot&1.8\,M_\odot&2.0\,M_\odot\\
\hline
{\rm mixed},~2.0~{\rm kpc}
&1.229&0.907&0.830\\
{\rm pure},~2.0~{\rm kpc}
&2.710&2.000&1.830\\
{\rm mixed},~2.65~{\rm kpc}
&2.158&1.592&1.457\\
{\rm pure},~2.65~{\rm kpc}
&4.758&3.512&3.213
\end{array}
\times10^{-15}~{\rm s\,s^{-1}}.
\label{eq:sm_mass_table}
\end{equation}
Increasing mass generally increases the available moment of inertia
on the certified branches and therefore lowers the required
\(\dot P_{\rm crit}\). The canonical-mass crossing is not a
mass-independent exclusion.

The reference spin-down is therefore a benchmark coordinate for the
boundary, not a measured intrinsic property of the source.

% ============================================================
\section{Engine closure and GeV consistency}
\label{sm:closure}

For the current mixed construction, the 1--25 TeV leptonic component
and 25--100 TeV hadronic component require
\begin{equation}
L_e
=
1.605\times10^{33}
~{\rm erg\,s^{-1}},
\end{equation}
and
\begin{equation}
L_p
=
2.665\times10^{33}
~{\rm erg\,s^{-1}},
\end{equation}
respectively, so that
\begin{equation}
L_{\rm inj}
=
4.270\times10^{33}
~{\rm erg\,s^{-1}}.
\end{equation}
At \(\dot P_{\rm ref}\), the certified
\(1.4\,M_\odot\) cohort spans
\begin{equation}
\dot E_{\rm sd}
=
(0.801-1.372)\times10^{34}
~{\rm erg\,s^{-1}},
\end{equation}
with median
\begin{equation}
\dot E_{\rm sd,med}
=
1.042\times10^{34}
~{\rm erg\,s^{-1}}.
\end{equation}
Hence
\begin{equation}
\frac{L_{\rm inj}}{\dot E_{\rm sd}}
=
0.311-0.533,
\qquad
\left(\frac{L_{\rm inj}}{\dot E_{\rm sd}}\right)_{\rm med}
=
0.410.
\end{equation}
Thus the mixed TeV--UHE injection budget closes over the full
canonical-mass cohort at the reference spin-down.

The phase-averaged GeV band imposes a separate necessary condition.
Using
\begin{equation}
G_{100}
=
4.1\times10^{-10}
~{\rm erg\,cm^{-2}\,s^{-1}}
\end{equation}
\cite{Zabalza2011}, the 2.0-kpc isotropic-equivalent luminosity is
\begin{equation}
L_{\rm GeV,iso}
=
1.96\times10^{35}
~{\rm erg\,s^{-1}}.
\end{equation}
Writing the actual luminosity entering the rotational budget as
\(f_\Omega L_{\rm GeV,iso}\), the median-EoS condition
\begin{equation}
f_\Omega L_{\rm GeV,iso}
\leq
\dot E_{\rm sd}
\end{equation}
requires
\begin{equation}
\dot P_{\rm GeV,min}
=
5.65\times10^{-14}f_\Omega
~{\rm s\,s^{-1}}
\label{eq:sm_gevpdot}
\end{equation}
at 2.0 kpc, or
\begin{equation}
\dot P_{\rm GeV,min}
=
9.91\times10^{-14}f_\Omega
~{\rm s\,s^{-1}}
\end{equation}
at 2.65 kpc. For \(f_\Omega=1\), these are respectively
18.8 and 33.1 times \(\dot P_{\rm ref}\).

At the UHE energetic crossing, the dependence on
\(I\), \(P\), and \(\dot P_{\rm rot}\) cancels from the ratio between
the required UHE-channel power and the GeV isotropic-equivalent
luminosity. In the current implementation,
\begin{equation}
f_{\Omega,\rm crit}^{\rm mixed}=0.02176,
\qquad
f_{\Omega,\rm crit}^{\rm pure}=0.04799.
\label{eq:sm_fomega}
\end{equation}
Thus the current mixed and pure UHE requirements correspond to
2.176\% and 4.799\%, respectively, of the isotropic-equivalent GeV
luminosity. These values are EoS independent because the common
stellar factors cancel algebraically.

If the GeV and UHE components are required to share the same
rotation-powered reservoir with \(f_\Omega\simeq1\), the GeV closure
condition pushes the intrinsic spin-down far above the UHE crossing.
In that regime the UHE energetic boundary ceases to discriminate
among the certified EoS. The GeV consistency test therefore does not
provide a second EoS ranking; it defines an engine-geometry condition
under which the UHE ranking is or is not physically relevant.

This establishes the engine-geometry condition under which the
\(I(M)\)-dependent energetic crossing derived above remains physically
relevant.

% ============================================================
\section{Energetic ordering and downstream tidal diagnostic}
\label{sm:structural_overlap}

At fixed mass and fixed source conditions,
Eq.~(\ref{eq:sm_inverseI}) shows that \(K_{\rm src}\) is common to all
EoS. Consequently, the critical-spin-down ordering is exactly
equivalent to ordering the EoS by decreasing \(I(M)\). Coherent
source-systematic shifts change \(K_{\rm src}\) and move the energetic
boundary, but cannot reorder the EoS. We therefore refer to this
quantity as an \emph{energetic EoS ordering}, not as a posterior
preference score.
\begin{table*}[t]
\centering
\caption{
Nine EoS in the central energetic--tidal overlap. The tidal criterion
is a downstream diagnostic and does not enter the energetic ordering.
The listed ranks are the pure-hadronic \(>1\) TeV, 2.0-kpc,
\(1.4\,M_\odot\) energetic ranks.
}
\label{tab:sm_nine}

\small
\begin{ruledtabular}
\begin{tabular}{c l l c c c c}
Rank & EoS & Class &
\(I_{45}(1.4)\) &
\(R_{1.4}\) [km] &
\(\Lambda_{1.4}\) &
\(\dot P_{\rm crit}\,[10^{-15}{\rm s\,s^{-1}}]\)\\
\hline
74 & SKa & Skyrme/nuclear & 1.6136 & 12.894 & 563.1 & 2.881\\
75 & V-QCD(APR), stiff & V-QCD/holographic & 1.6087 & 12.549 & 552.0 & 2.890\\
76 & PCSB2 & RMF/hadronic & 1.6051 & 12.895 & 551.2 & 2.896\\
77 & SPG(M1) & QHC/crossover & 1.5919 & 12.790 & 532.6 & 2.920\\
78 & STOS-TM1-v2-T0 & RMF/hadronic & 1.5907 & 11.950 & 530.6 & 2.922\\
79 & SPG(M2) & QHC/crossover & 1.5820 & 12.624 & 520.0 & 2.938\\
80 & Brussels-Montreal BSk24 & Skyrme/nuclear & 1.5785 & 12.576 & 516.3 & 2.945\\
81 & V-QCD(APR), intermediate & V-QCD/holographic & 1.5704 & 12.416 & 504.6 & 2.960\\
82 & SkI6 & Skyrme/nuclear & 1.5553 & 12.469 & 489.2 & 2.989\\
\end{tabular}
\end{ruledtabular}
\end{table*}
At \(M=1.4\,M_\odot\), \(d=2.0\) kpc, and
\(\dot P_{\rm ref}\), the central pure-hadronic \(>1\) TeV energetic boundary is
satisfied by 82 of the 116 certified EoS. In a separately applied
downstream test, 43 of 116 satisfy the diagnostic
\begin{equation}
\Lambda_{1.4}\leq580.
\end{equation}
Their intersection contains nine EoS,
\begin{equation}
N_{\rm energy}=82,\qquad
N_{\rm tidal}=43,\qquad
N_{\rm both}=9,\qquad
N_{\rm neither}=0.
\end{equation}
These are counts over the working library, not probabilities or
allowed fractions of the physical EoS population.

The nine EoS occupy energetic ranks 74--82 and are listed in
Table~\ref{tab:sm_nine}. They span different microscopic model classes,
so the intersection identifies a narrow structural region rather than
a unique preferred microphysical family. Across the nine models,
\begin{equation}
1.555\leq I_{45}(1.4)\leq1.614,
\end{equation}
\begin{equation}
11.95\leq R_{1.4}\leq12.90~{\rm km},
\end{equation}
and
\begin{equation}
489\leq\Lambda_{1.4}\leq563.
\end{equation}
Their central energetic boundaries lie in the narrow interval
\begin{equation}
2.881\times10^{-15}
\leq
\dot P_{\rm crit}
\leq
2.989\times10^{-15}
~{\rm s\,s^{-1}},
\end{equation}
close to \(\dot P_{\rm ref}\). Under the coherent unfavorable
instrumental envelope, the same structural region is shifted to
approximately
\begin{equation}
3.29\times10^{-15}
\lesssim
\dot P_{\rm crit}
\lesssim
3.42\times10^{-15}
~{\rm s\,s^{-1}},
\end{equation}
showing that the nine-model central overlap is a boundary region rather
than a systematic-independent exclusion set.



The nine-model intersection is passed to
Sec.~\ref{sm:microphysics} only for structural visualization; it is not
used to redefine the energetic ordering.

% ============================================================
\section{Structural and microphysical visualization}
\label{sm:microphysics}

Figure~\ref{fig:uhe_boundary_structure}(a1) displays the certified branch-resolved mass--radius
sequences in gray and overlays the nine audited intersection EoS in
color. The NICER and GW170817 information shown there is observational
context only and does not modify the UHE energetic ranking.

For the nine highlighted EoS, Fig.~\ref{fig:uhe_boundary_structure}(a2) reconstructs the thermodynamic
profiles directly from the original barotropic source bundles. The
displayed sound speed is the raw derivative
\begin{equation}
c_{s,\rm raw}^2
=
\frac{dP}{d\varepsilon}
=
\frac{P/\varepsilon}
{d\ln\varepsilon/d\ln P},
\end{equation}
without clipping to the causal interval for visualization. The
horizontal lines at \(c_s^2=1/3\) and \(c_s^2=1\) are reference lines
only; they are not additional ranking weights or post-hoc filters.
The pressure curves \(P(\varepsilon)\) are shown on the secondary axis,
and the colored markers indicate the central energy density reached by
the corresponding \(1.4\,M_\odot\) TOV solution.

The compact \(I_{45}\)--\(\Lambda_{1.4}\) panel uses the continuous
\(I\)--Love relation only as a structural guide. The energetic
threshold \(I_{45,\rm crit}=1.5504\) and separately applied tidal threshold
\(\Lambda_{1.4}=580\) delimit the central overlap. The nine colored
points identify the audited EoS in that overlap; they are not used to
fit the relation.

Thus Fig.~\ref{fig:uhe_boundary_structure}(a1,a2,d2,e) visualizes
quantities that are downstream of the energetic calculation; none is
fed back into \(f_{\rm joint}\) or \(\dot P_{\rm crit}\).


% ============================================================
\section{Statements intentionally not made}
\label{sm:not_claimed}

The present analysis does not interpret the UHE data as a universal
EoS selector. In particular:

\begin{enumerate}
\item no TOV or Love observable modifies the orbital acceleration or
      \(\gamma\gamma\)-transparency conditions;
\item no radius, tidal-deformability, maximum-mass, or sound-speed
      score is multiplied into the UHE energetic boundary;
\item EoS counts are bookkeeping results for the tested library and
      are not posterior probabilities;
\item common source systematics shift the energetic boundary but do
      not provide independent evidence for rank stability, because the
      fixed-mass ordering is algebraically the inverse-\(I\) ordering;
\item the nine-model energetic--tidal intersection is a structural
      overlap across multiple microscopic families, not evidence for a
      unique preferred family;
\item the pure-hadronic \(>1\) TeV construction is a limiting stress test, not a
      preferred emission model or an observationally inferred EoS cut;
\item if the phase-averaged GeV component shares the same rotational
      reservoir with \(f_\Omega\simeq1\), the direct GeV closure
      condition removes the UHE EoS discrimination.
\end{enumerate}


\end{document}
